# Supplementary material for: F$^{2}$-NeRF: Fast Neural Radiance Field Training with Free Camera Trajectories
Source: arXiv:2303.15951 source file (2023-03-28)
Supplement: Supplementary file 1 [file supp_impl_lin_matrix.tex]

\begin{figure}[htb]
  \includegraphics[width=\linewidth]{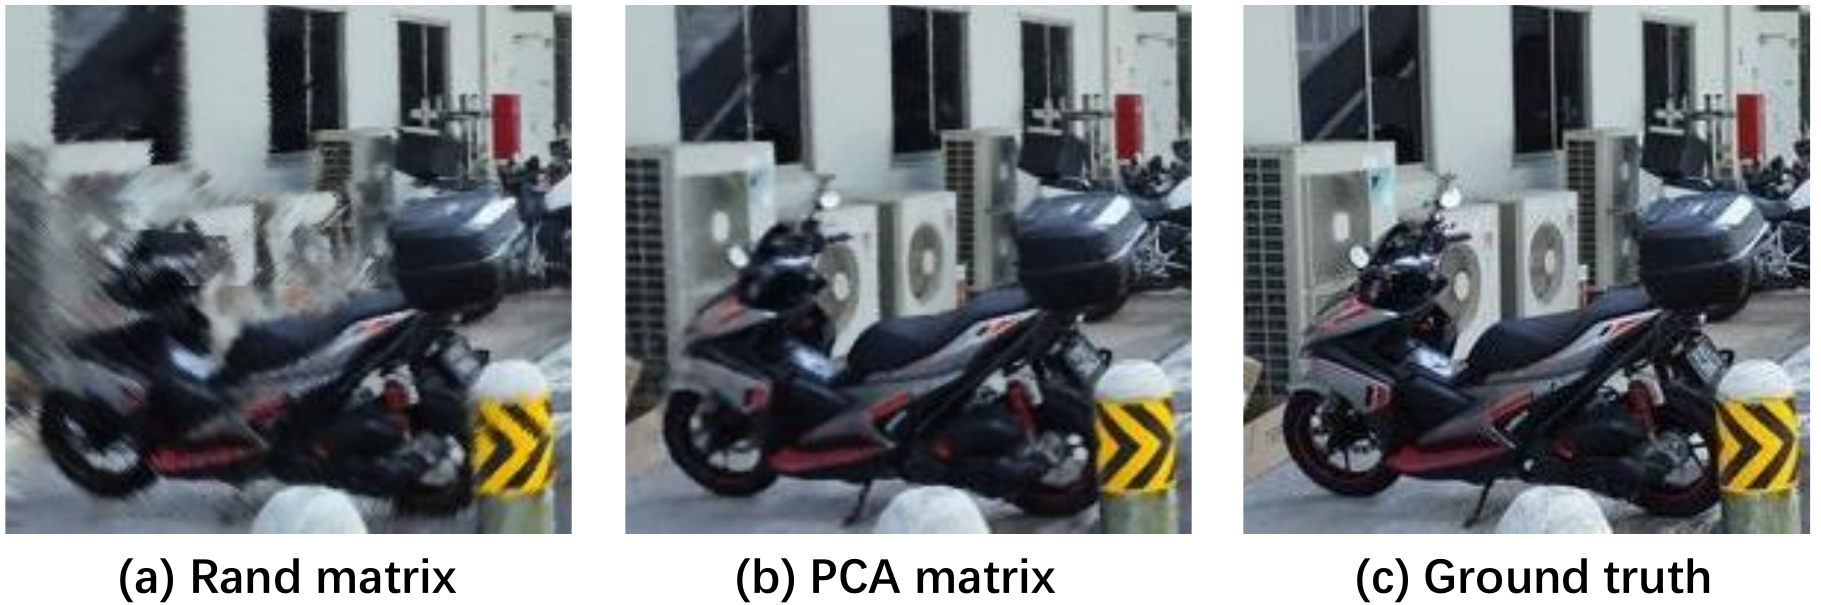} \caption{{\bf Visual comparison between using rand matrix~(a) and using PCA matrix~(b).}}
  \label{fig:lin_matrix}
\end{figure}
